# Supplementary material for: Doubly Modulated Optical Lattice Clock Interference and Topology
Source: arXiv:2009.11671 source file (2021-07-14)
Supplement: Supplementary file 1 [file SM.pdf]

# Supplementary Material of
# "Doubly Modulated Optical Lattice Clock: Interference and Topology"

Xiao-Tong Lu,[1,2,*] Tao Wang,[3,*] Ting Li,[1,2] Chi-Hua Zhou,[1,2] Mo-Juan Yin,[1,2] Ye-Bing Wang,[1,2] Xue-Feng Zhang,[3,†] and Hong Chang[1,2,‡]

[1]*Key Laboratory of Time and Frequency Primary Standards, National Time Service Center, Chinese Academy of Sciences, Xi'an 710600, China*
[2]*School of Astronomy and Space Science, University of Chinese Academy of Sciences, Beijing 100049, China*
[3]*Department of Physics, and Center of Quantum Materials and Devices, Chongqing University, Chongqing, 401331, China*

In the Supplemental Material, we presents more details about the experimental realizations, Floquet methods, driving stability, Frequency shift , Eigen-energy measurement and uncertainty of $K_c$.

**Experimental Realization.** The lattice laser is generated by an external cavity semiconductor laser (TA PRO), and its frequency can be modulated by adding sinusoid signal $\mathrm{S_F}(t)$ to the piezo-electric transducer (PZT) pasted on the grating which is used for tuning the laser frequency. Based on previous work [1], the response of PZT is quite linear, so the frequency is modulated approximately following the signal $\mathrm{S_F}(t)$. After two steps Doppler cooling processes, the temperature is decreased down to $\approx 3\ \mu K$. The transverse and longitude frequencies of harmonic trap are $\nu_r = 250$ Hz and $\nu_z = 62.5$ kHz, respectively. Thus, the numbers of external energy levels considered are $n_r \approx 1000$ and $n_z \approx 5$.

The wavelength of clock laser is $\lambda_p \approx$698 nm, and it is aligned along the same direction as lattice laser with tiny misaligned angle $\delta\theta = 9$ mrad. The beam-waist radius of the clock laser is $W_C \approxeq$ 1mm, while the waist radius of the lattice laser is much smaller $W_L \approxeq 50\mu$m. For the Gaussian beam laser, the amplitude of field is $E(r,z) = E_0 \frac{W_C}{W(z)} e^{-\frac{r^2}{W(z)^2}}$, in which $E_0$ is the field strength at the center of the lattice where $(r,z) = (0,0)$ and $W(z) = W_C\sqrt{1+(z/z_R)^2}$ is the radius at position $z$ with Rayleigh length $z_R = \pi W_C^2/\lambda_p = 4.5m$. Because the Rabi frequency $\Omega(z,r)$ is proportional to the field $E(r,z)$, it could be written as $\Omega(z,r) = \Omega_0 \frac{W_C}{W(z)} e^{-\frac{r^2}{W(z)^2}}$, where $\Omega_0/2\pi \approxeq 9.0$Hz is the Rabi frequency at the center of lattice. The size of the magneto-optical trap (MOT) is $W_{\mathrm{MOT}} = 0.5$mm, so the weakest Rabi frequency is at $(r,z) = (W_L, W_{\mathrm{MOT}}/2)$ and the ratio is $\Omega(W_L, W_{\mathrm{MOT}}/2)/\Omega_0 \approxeq 0.9975$. Therefore, the inhomogeneity induced by different position can be omitted.

As shown in Fig.1 (a), an acoustic optical modulator (AOM) is used for simultaneously modulating both frequency and intensity of the clock laser. Two sinusoidal waveform signals with relative phase $\phi$ are generated by an arbitrary function generator (AFG, Tektronix AFG3000), and both of them are input into a microwave switch (MS) controlled by square waveform signal $\mathrm{S_r}(t)$ with frequency $\omega_s/2\pi$. Then, additional sinusoidal waveform signal $\mathrm{S_{PW}}(t)$ is fed into a voltage variable attenuator (VVA), so that the amplitude of input signal with phase modulation $f(t)$ (Eq. (4)) is also modulated. Finally, the output signal from VVA is imposed into AOM to carry out the transverse modulation.

Three signals ($\mathrm{S_F}(t)$, $\mathrm{S_r}(t)$ and $\mathrm{S_{PW}}(t)$) are generated from one function generator which is a data acquisition (DAQ, NI USB-6341) card. Thus, the signals $\mathrm{S_r}(t)$ and $\mathrm{S_{PW}}(t)$ can be synchronized without additional synchronous signal during the transverse modulation. Meanwhile, the relative phase between three signals can be well controlled during the double modulation.

**Floquet method.** Dealing with Eq.(3) of main text, we first go to interaction picture by constructing unitary operator $\hat{U}_1 = e^{-i\frac{\Delta t}{2\hbar}\sigma_z}$. With $\hat{U}_1^\dagger(\hat{H}_T - i\hbar\frac{\partial}{\partial t})\hat{U}_1$ and rotating wave approximation (RWA), we can get for each period:

$$\hat{H}_{I_T} = \hbar \begin{cases} \frac{\Omega_{\vec{n}}}{4}\left(e^{i(\delta-\omega_s)t} + e^{i(\delta+\omega_s)t}\right)\sigma_+ + h.c. \\ \frac{\Omega_{\vec{n}} e^{i(\pi-\phi)}}{4}\left(e^{i(\delta-\omega_s)t} + e^{i(\delta+\omega_s)t}\right)\sigma_+ + h.c. \end{cases} \tag{1}$$

We could see clearly in the interactive picture that the hopping amplitude of $\sigma_+$ is given an additional phase $\pi - \phi$ in half of the period, while at the other half this phase is zero, as shown in Fig.2a. In the resolve sideband approximation that $\hbar\omega_s \gg g_{\vec{n}}$, with $|\delta - n_t\omega_s| \ll \omega_s$, one only needs to consider $n_t$th Floquet sideband, we transform back with the unitary operator $\hat{U}_2 = e^{i\frac{\delta - n_t\omega_s}{2}\sigma_z}$, and get

$$\hat{H}_T^{n_t} = \hat{H}_d + \frac{\hbar\Omega_{\vec{n}}}{4}\begin{cases} e^{in_t\omega_s t}\cos(\omega_s t)\sigma_+ + h.c. \\ e^{i(n_t\omega_s t + \pi - \phi)}\cos(\omega_s t)\sigma_+ + h.c. \end{cases} \tag{2}$$

in which $\hat{H}_d = \frac{\hbar(\delta - n_t\hbar\omega_s)}{2}\sigma_z$ is the diagonal part. Because the driving character energy $\omega_s$ are much larger than the energy scale $(\delta - n_t\hbar\omega_s), \Omega_{\vec{n}}$ in Hamiltonian $\hat{H}_T^{n_t}$ , we could use Floquet-Magnus expansion to get the lowest order effective Hamiltonian $\hat{H}_e = 1/T\int_0^T \hat{H}(t)dt$ that

$$\hat{H}_{Te}^{n_t} = \frac{\hbar(\delta - n_t\hbar\omega_s)}{2}\sigma_z + \left(\frac{\hbar\Omega_{\vec{n}}^{n_t}}{2}\sigma_+ + h.c.\right), \tag{3}$$

in which the effective Rabi frequency of $n_t$th Floquet sideband at external state $\vec{n}$ is $\Omega_{\vec{n}}^{n_t}$.

For double modulation, the time periodically Hamiltonian after RWA approximation could be written as

$$\hat{H}_D = \frac{\delta + A\cos(\omega_s t + \psi)}{2}\hbar\sigma_z + \frac{\hbar\Omega_{\vec{n}}}{2}\cos(\omega_s t)\sigma_x, \quad (4)$$

which could be transformed to the interaction picture by the unitary operator $\hat{U}_3 = e^{-i\frac{\delta t-(A/\omega)\sin(\omega_s t+\psi)}{2}}$ and get:

$$\hat{H}_{I_D} = \frac{\hbar\Omega_{\vec{n}}}{4}\left[e^{i[(\delta+\omega_s)t+A\sin(\omega_s t+\psi)]} + e^{i[(\delta-\omega_s)t+A\sin(\omega_s t+\psi)]}\right]\sigma_+ + h.c.. \quad (5)$$

If $|\delta - n_t\hbar\omega_s| \ll \omega_s$ and the resolved sideband approximation is taken, only $n_t$th sideband needs to be considered, thus we could transform back with $\hat{U}_2 = e^{i\frac{\delta-n_t\omega_s}{2}\sigma_z}$ and get

$$\hat{H}_D^{n_t} = \frac{\hbar(\delta - n_t\hbar\omega_s)}{2}\sigma_z + \frac{\hbar\Omega_{\vec{n}}}{4}\left[e^{i[(n_t+1)\omega_s t+A\sin(\omega_s t+\psi)]}\sigma_+ + e^{i[(n_t-1)\omega_s t+A\sin(\omega_s t+\psi)]}\sigma_+ + h.c.\right]. \quad (6)$$

Also using Jacobi-Anger relation $e^{iK\sin(\omega_s t+\psi)} = \sum_n J_n[K]e^{in\omega_s t+in\psi}$ and Floquet-Magnus expansion to get the lowest order effective Hamiltonian

$$\hat{H}_{De}^{n_t} = \frac{\hbar\delta - n_t\hbar\omega_s}{2}\sigma_z + \frac{\hbar\Omega_{\vec{n}}}{4}\left[\left(J_{n_t-1}[K]e^{i(n_t-1)\psi} + J_{n_t+1}[K]e^{i(n_t+1)\psi}\right)\sigma_+ + h.c.\right], \quad (7)$$

in which $K = A/\omega_s$ is the renormalized driving amplitude.

**Driving stability.** For the Floquet spectroscopy, the driving frequency is usually very high, such as kHz in shaking optical lattice [2]. However, in order to stabilize the relative phase, the driving frequency has to be low which requires very narrow line-width of spectrum. The ultra-high precision and ultra-stability of OLC make the Floquet sideband can be clear resolved even at driving frequency equal to 100Hz (comparing with kHz in Ref.[2]), so that fine-tuning both modulation at such low frequency becomes technically easy (but building OLC is extremely hard). The stability of phase is highly related to the synchronization of all signals and also their frequency stability. Because all driving signals are generated by the USB-6341 in our system, they are naturally synchronized and their stabilities are same as USB-6341.

In order to test the instability of the relative phase, we compare Rabi spectrum for different driving frequency $\omega_s$ =100Hz, 200Hz and 300Hz respectively for the same relative phases and the same driving amplitude, and the stabilities of different driving frequency are shown in Figure S1. As shown in Figure S2 of SM, the experimental and theoretical results matches very well. The Rabi

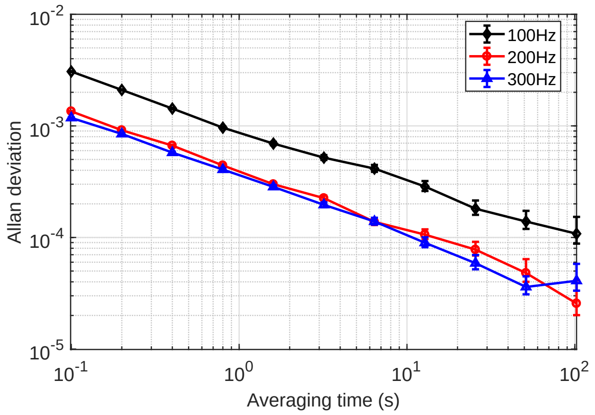


Figure S1: The stability of the USB 6341 at different output frequency.

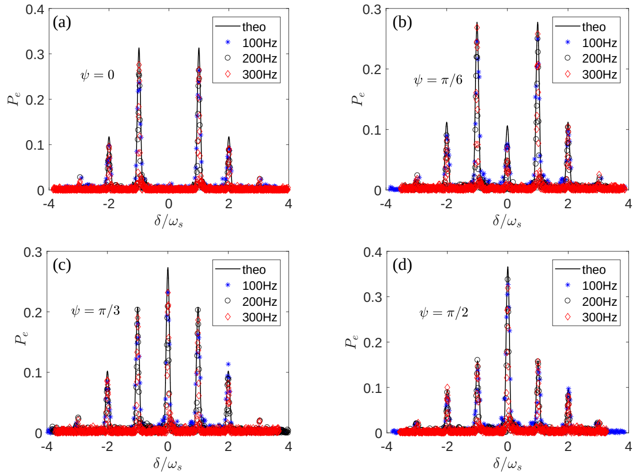


Figure S2: Rabi spectrum for different relative phase at driving frequency $\omega_s$ =100Hz, 200Hz and 300Hz respectively. All the other parameters are the same as Figure 3 in main text except $K = 1.1$, and the detuning $\delta$ is rescaled with unit of $\omega_s$.

spectrum is only related to relative phase if we rescale detuning $\delta$ with unit of $\omega_s$, which is consistent with our theoretical calculation (Eq.(7) in main text). If the instability of the relative phase is highly relevant, it will strongly change the spectrum at high driving frequency.

**Frequency shift.** The independence of atoms can be checked via estimate of the state-dependent mean-field shift. The s-wave frequency shift can be roughly estimated with

$$\Delta\nu_s = \nu_0(\Delta\Omega/\bar{\Omega})^2, \quad (8)$$

where $\nu_0 = 2\hbar\rho_0 a_{eg}/m$, with the mass of atom $m$, the s-wave scattering length $a_{eq}$ and the average atom density $\rho_0$ [3, 4]. The s-wave scattering length $a_{eg}$ is equal to $69a_0$

($a_0$ is the Bohr radius) [5], and the average atom density is $\rho_0 \approxeq 1.9 \times 10^{17}/m^3$ [6], so we can obtain $\nu_0 \approxeq 1.01$Hz.

After that, we check the inhomogeneity $\Delta\Omega/\bar{\Omega}$ which can be calculated via

$$\bar{\Omega} = \sum_{n_z,n_r} q_{n_z} q_{n_r} \Omega_{n_z,n_r}, \tag{9}$$

$$\Delta\Omega = \sum_{n_z,n_r} q_{n_z} q_{n_r} \Omega^2_{n_z,n_r} - \bar{\Omega}^2, \tag{10}$$

where $q_{n_z}(q_{n_r})$ is the normalized Boltzmann weights corresponding to transverse (longitudinal) temperature and $\Omega_{n_z,n_r}$ is the Rabi frequency in different motional state. Substituting $T_r = 2.9\mu K$, $T_z = 2.7\mu K$, $\nu_r = 250$Hz, $\nu_z = 62.5$kHz, $N_r = 1000$ and $N_z = 5$ into equations above, we can get $\Delta\Omega/\bar{\Omega} \approxeq 0.34$. Then, we can get **the s-wave mean field shift $\Delta\nu_s$ is about 0.12Hz** (The effect of excitation fraction usually decreases the s-wave mean-field shift, so here $\Delta\nu_s$ can be taken as an estimation of maximum value).

On the other hand, the frequency density shift contributed by the p-wave collisions is larger. Basing on the Ref.[7, 8], the frequency shift can be roughly calculated via

$$\Delta\nu_p = N_s(C - \chi(2f-1)), \tag{11}$$

where $C = (V^{ee} - V^{gg})/2$ and $\chi = (V^{gg} + V^{ee} - 2V^{gg})/2$, $V^{gg}$, $V^{ee}$ and $V^{gg}$ represent p-wave interaction parameters between the three possible electronic symmetric states $|gg\rangle$, $|ee\rangle$ and $\frac{1}{\sqrt{2}}(|ge\rangle + |eg\rangle)$, $f \in [0,1]$ is the excitation fraction, and $N_s$ is the average number of atoms in each site. The p-wave interaction parameters can be explicitly written as

$$V^{\alpha\beta} = v^{\alpha\beta} \sum_{\vec{n},\vec{n}'} P_{\vec{n},\vec{n}'}, \tag{12}$$

where $P_{\vec{n},\vec{n}'}$ is characterize p-wave matrix which is almost temperature independent and related to the harmonic oscillator modes in different motional state $\vec{n}$ and $\vec{n}'$, and $v^{\alpha\beta} = \frac{b^3_{\alpha\beta}}{a^z_{ho} a^r_{ho}{}^4}$ with p-wave scattering length $b^{\alpha\beta}$ and the harmonic oscillator length $a^{z(r)}_{ho} = \sqrt{\frac{\hbar}{2\pi m \nu_{z(r)}}}$. In the Ref.[7], the coefficients in Eq.(11) is extracted from the measurement as $\chi' = 2\pi \times 0.20(4)$ and $C' = -0.3\chi'$ with frequency $\nu'_r = 450$Hz and $\nu'_z = 80$kHz, so in our platform with $\nu_r = 250$Hz and $\nu_z = 62.5$kHz, the coefficient can be roughly obtained by $\chi = \chi'(\nu_r/\nu'_r)^2\sqrt{\nu_z/\nu'_z} \approx 0.34$Hz and $C = -0.3\chi$ (p-wave matrix $P_{\vec{n},\vec{n}'}$ is unchanged). Then, considering $N_s \approx 40$ and $f \in [0,1]$, we can get **the p-wave mean field shift $\Delta\nu_p$ is about** $[-2.88, 1.55]$**Hz.** Then, because the total mean field shift is less than 3Hz, the assumption of independent atoms is reasonable.

**Eigen-energy measurement.** As statement in the main text, the $n_d$th sideband effective Floquet Hamiltonian could be taken as spin 1/2 atom coupled to two magnetic fields $H^{n_d}_{\rm EF} = \frac{\hbar}{2}\vec{h}_{n_d}\cdot\vec{\sigma}$ with $\vec{h}_{n_d} = \vec{B}_{n_d-1} + \vec{B}_{n_d+1}$ and $\vec{B}_{n_d} = \frac{\Omega_{\vec{n}} J_{n_d}[K]}{2}\{\cos(n_d\psi), -\sin(n_d\psi), \frac{\delta - n_d\omega_s}{\Omega_{\vec{n}} J_{n_d}[K]}\}$. If we consider $h^z_{n_d} = 0$ where the peak of $n_d$th order Floquet sideband stands, the effective magnetic field lays down in the XY plane and the model changes into

$$H^{n_d}_{\rm EF} = \frac{\hbar}{2}\left(h^x_{n_d}\sigma^x + h^y_{n_d}\sigma^y\right), \tag{13}$$

with eigen-energy equal to $E^{\pm}_{n_d}(\psi) = \pm\frac{\hbar}{2}\sqrt{(h^x_{n_d})^2 + (h^y_{n_d})^2} = \pm\frac{\hbar}{2}|\vec{h}_{n_d}|$.

In experiment, the eigen-energy can be obtained by measuring the Rabi oscillation. The atoms are prepared in the ground state, and the initial wave-function is $\psi_0 = |g\rangle$. Then, the wave-function is $\psi(t) = \exp(-iH^{n_d}_{\rm EF}t/\hbar)\psi_0$, so the probability of internal excited states is

$$P_e(t) = \sin^2\left(\frac{\sqrt{(h^x_{n_d})^2 + (h^y_{n_d})^2}}{2}t\right) = \sin^2\left(\frac{|\vec{h}_{n_d}|}{2}t\right). \tag{14}$$

Because time evolution of the internal excited state is the same as the Rabi oscillation, the effective Rabi-frequency is just equal to twice eigen-energy divided by $\hbar$.

**Uncertainty of $K_c$.** In order to experimentally obtain the uncertainty of the critical $K$, we make a long time measurement (400 ms) of Rabi spectra at different K around the expectation value. As shown in Figure S3(a), the 1st order Floquet side-band peaks are recognizable at two neighbor values $K = 1.758$ and $K = 1.926$, but buried in the noise at their mid-point $K = 1.842$. Moreover, after Lorenz fitting, both fitting lines of $K = 1.758$ and $K = 1.926$ nearly coincide. Thus, we take $K = 1.842$ as the critical value of 1st order Floquet sideband with maximum uncertainty 0.084. Meanwhile, the Figure S3(b) indicates $K = 3.10$ is the critical value of 2nd order Floquet sideband with maximum uncertainty 0.11.

* These authors contributed equally to this work.
† zhangxf@cqu.edu.cn
‡ changhong@ntsc.ac.cn

[1] Mo-Juan Yin, Tao Wang, Xiao-Tong Lu *et al* Chin. Phys. Lett. **38**, 073201 (2021)
[2] H. Lignier, C. Sias, D. Ciampini, Y. Singh, A. Zenesini, O. Morsch, and E. Arimondo, Phys. Rev. Lett. **99**, 220403 (2007).
[3] S. Blatt, J. W. Thomsen, G. K. Campbell, A. D. Ludlow, M. D. Swallows, M. J. Martin, M. M. Boyd, and J. Ye., Phys. Rev. A **80**, 052703(2009).
[4] G. K. Campbell *et al.*, Science **324**, 360 (2009).
[5] A. Goban, *et al.*, Nature **563**, 369C373 (2018).
[6] M. D. Swallows, IEEE Trans. Ultrason., Ferroelect., Freq. Contr. **59**, 416C425. (2012).
[7] M. J. Martin, M. Bishof, M. D. Swallows, X. Zhang, C. Benko, J. von Stecher, A. V. Gorshkov, A. M. Rey, and J. Ye. Science, **341**, 632, (2013).

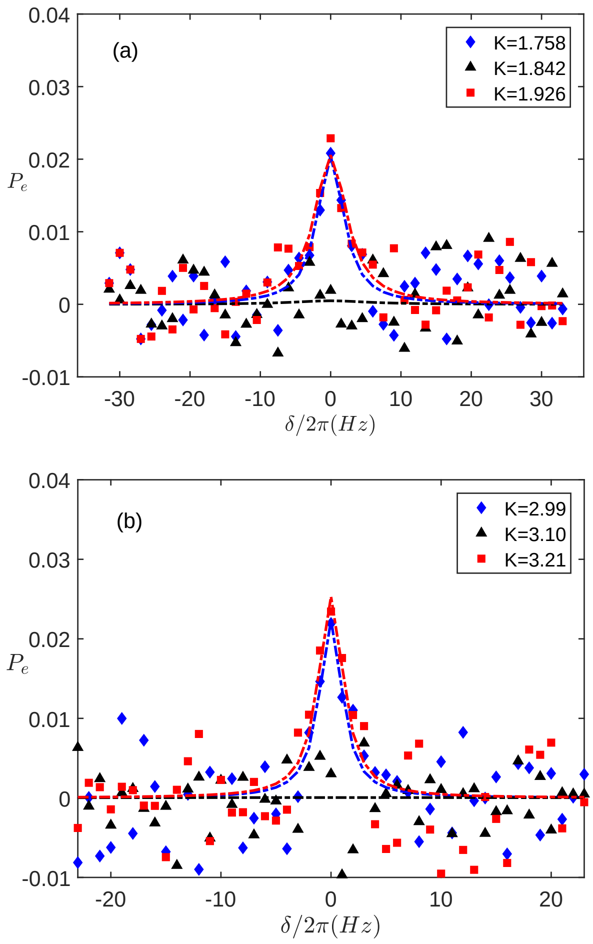


Figure S3: The Rabi spectra of the double modulation of the 1st order (a) and 2nd order (b) Floquet sideband at measuring time $t = 400$ms. The dots are experimental data and the dash lines are after Lorenz fitting.

[8] A. M. Rey, A. V. Gorshkov, C. V. Kraus, M. J. Martin, M. Bishof, M. D. Swallows, X. Zhang, C. Benko, J. Ye, N.D. Lemke, and A. D. Ludlow. Ann. Phys., **340** 311, (2014).
